# Supplementary material for: EdgeGFL: Rethinking Edge Information in Graph Feature Preference Learning
Source: arXiv:2502.02302 source file (2025-02-04)
Supplement: Supplementary file 1 [file B-9-Appendices.tex]

\appendices
\section{}
